# Supplementary material for: CLIPtone: Unsupervised Learning for Text-based Image Tone Adjustment
Source: arXiv:2404.01123 source file (2024-04-01)
Supplement: Supplementary file 4 [file sup_fig3_examples1.tex]

\begin{figure*}[t]
    \centerline{\includegraphics[width=0.95\textwidth]{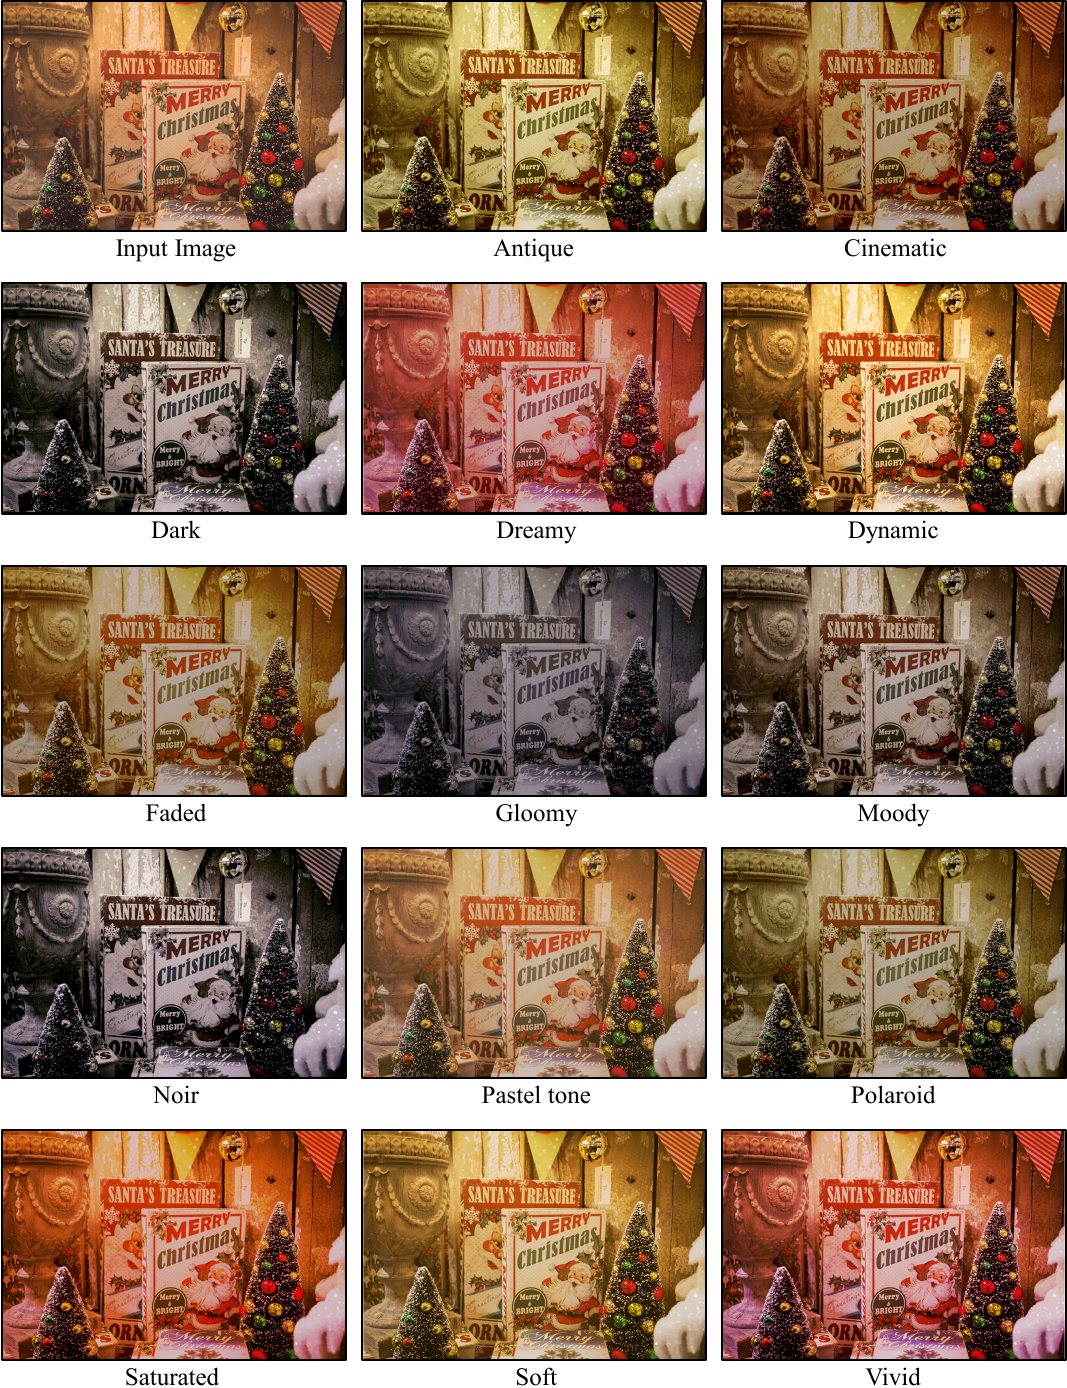}}
    \caption{
    Additional results of \MethodName{} with various text descriptions.
    }
    \label{fig:sup_fig3_examples1}
\end{figure*}
